# Supplementary material for: Explain and Predict, and then Predict Again
Source: arXiv:2101.04109 source file (2021-02-04)
Supplement: Supplementary file 1 [file a.appendix.tex]

\clearpage
\appendix

\section{Details on the effect of $\lambda$}
\label{sec:detailed-lambda-sweep}
In this section we present performance variation of both classification and explanation tasks in \mtlhard in figures \ref{fig:fever_lambda_sweep}, \ref{fig:movie_lambda_sweep} and \ref{fig:multirc_lambda_sweep}. Changes of our criteria of selecting the best $\lambda$-s are also presented in these figures. All results are based on model performance on the validation set.

\begin{figure*}[tb]
  \centering 
  \subfigure[Classification Macro Average F1]{ 
    \includegraphics[width=0.48\textwidth]{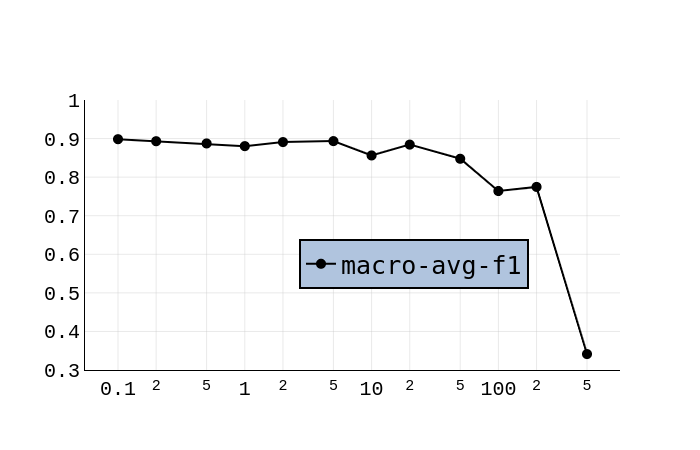}}
  \subfigure[comprehensiveness and sufficiency]{ 
    \includegraphics[width=0.48\textwidth]{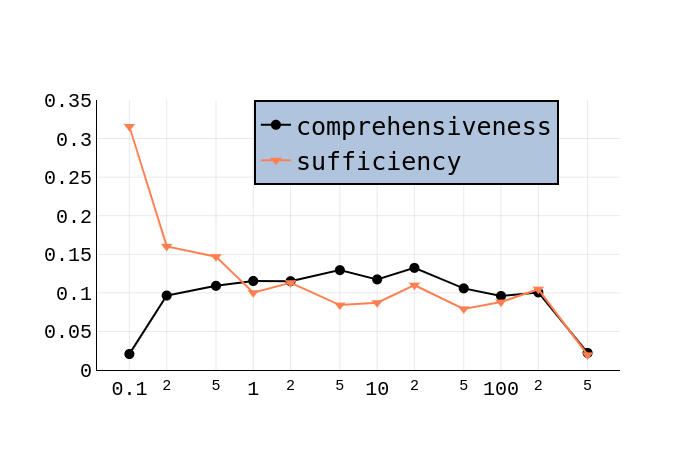}}
  \subfigure[AUPRC]{ 
    \includegraphics[width=0.48\textwidth]{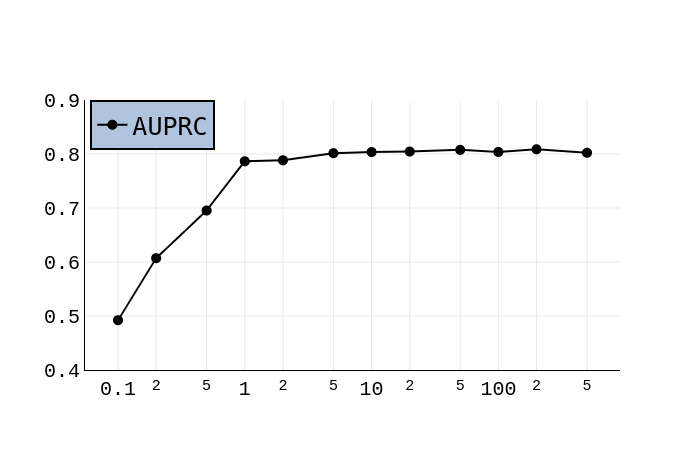}}
  \subfigure[Macro F1]{ 
    \includegraphics[width=0.48\textwidth]{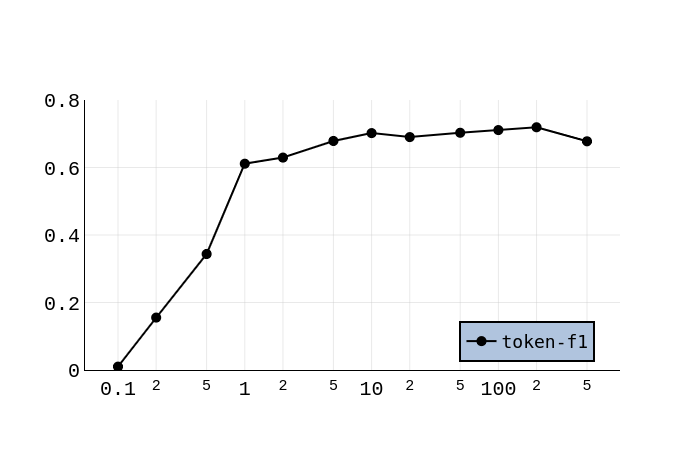}}
  \subfigure[$\lambda$-selection criteria for \mtlhard ]{ 
    \includegraphics[width=0.48\textwidth]{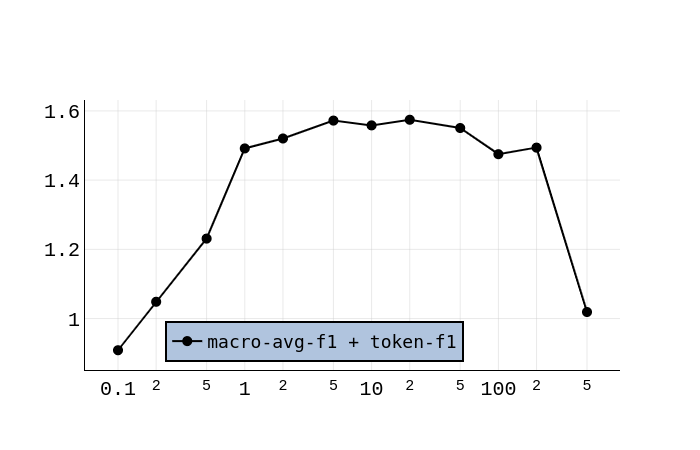}}
  \subfigure[$\lambda$-selection criteria for \mtlsoft]{ 
    \includegraphics[width=0.48\textwidth]{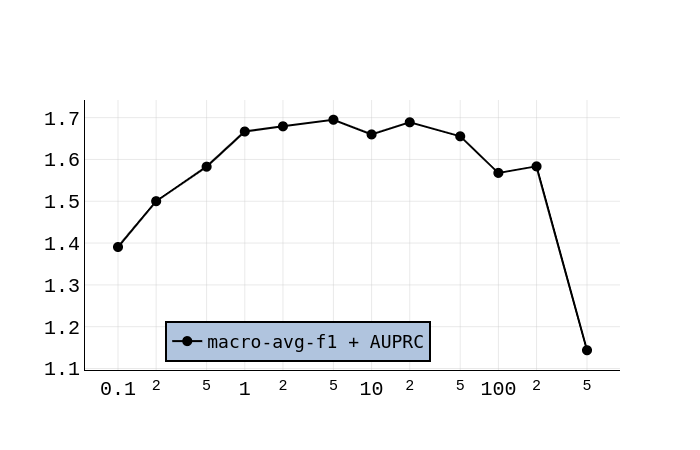}}
  \caption{Performance of task (a), explanation (b, c, d) and our $\lambda$ selection criteria for \mtlhard~and \mtlsoft~(e, f) with $\lambda$ (log-scale) on the validation set of \fever. Models for parameter-sweeping is trained on 10\% of the training set.}
  \label{fig:fever_lambda_sweep}
\end{figure*}

\begin{figure*}[t]
  \centering 
  \subfigure[Classification Macro Average F1]{ 
    \includegraphics[width=0.48\linewidth]{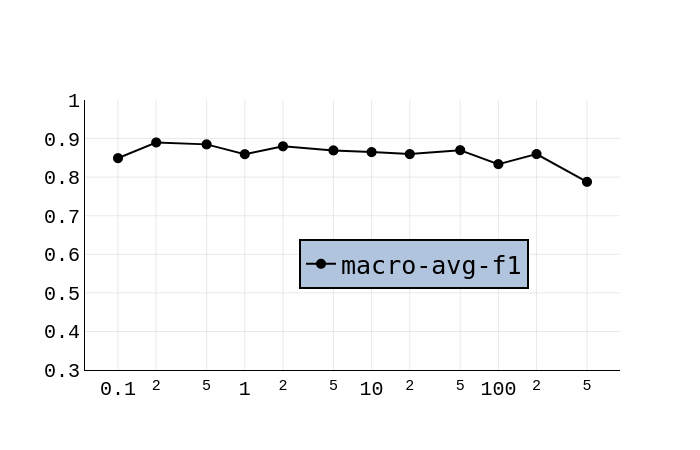}}
   \subfigure[comprehensiveness and sufficiency]{ 
     \includegraphics[width=0.48\linewidth]{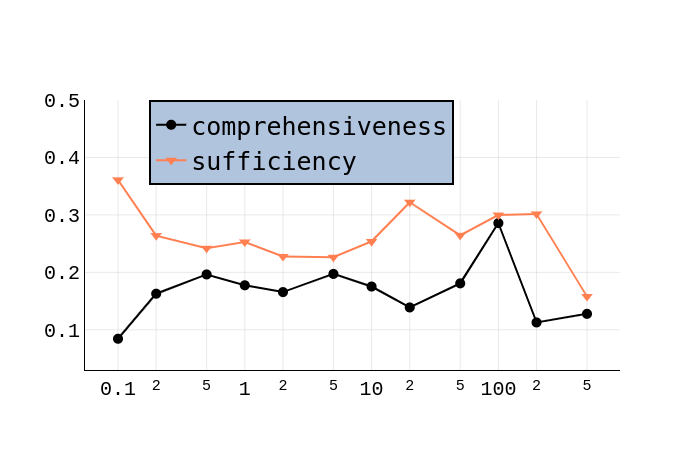}}
   \subfigure[AUPRC]{ 
     \includegraphics[width=0.48\linewidth]{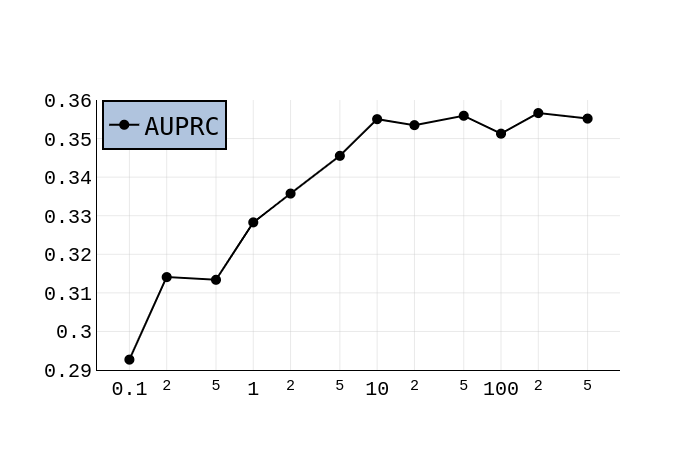}}
  \subfigure[Macro F1]{ 
    \includegraphics[width=0.48\linewidth]{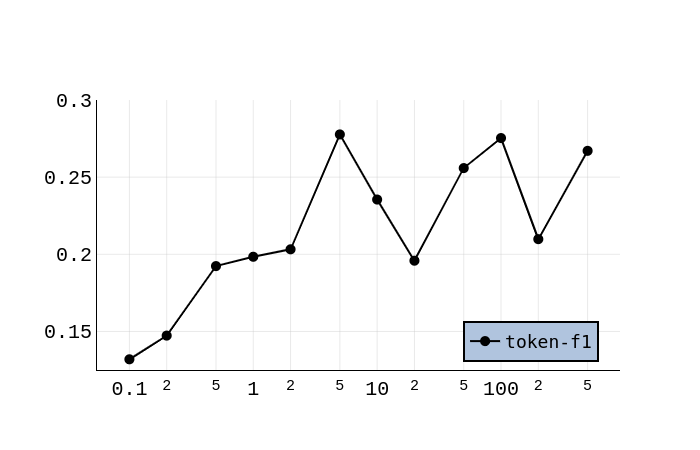}}
  \subfigure[$\lambda$-selection criteria for \mtlhard ]{ 
    \includegraphics[width=0.48\textwidth]{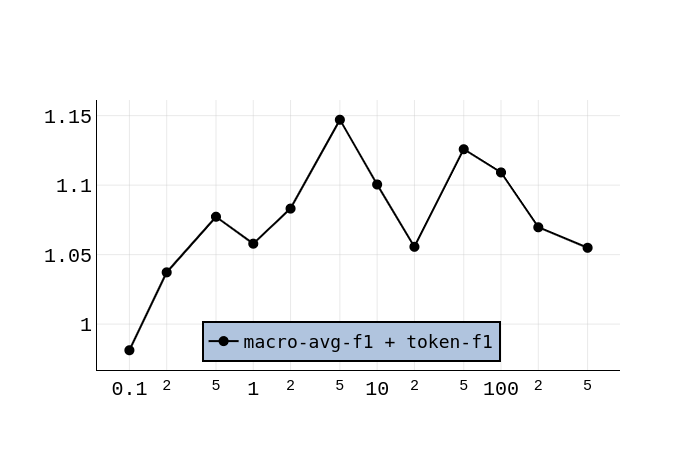}}
  \subfigure[$\lambda$-selection criteria for \mtlsoft]{ 
    \includegraphics[width=0.48\textwidth]{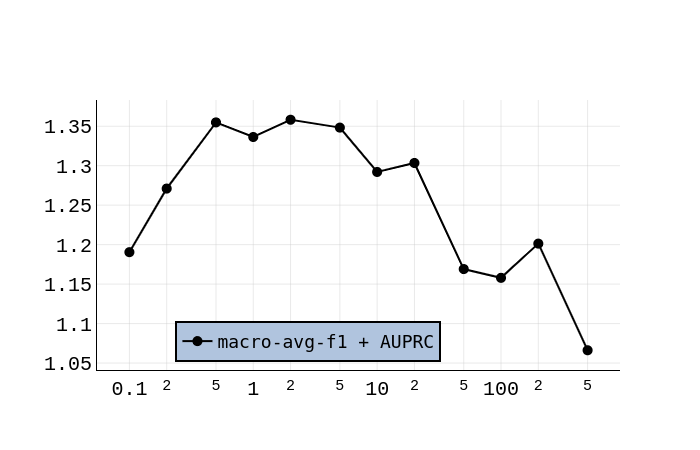}}    
    \caption{Performance of task (a), explanation (b, c, d) and our $\lambda$ selection criteria for \mtlhard~and \mtlsoft~(e, f) with $\lambda$ (log-scale)  on the validation set of \movie.}
  \label{fig:movie_lambda_sweep}
\end{figure*}

\begin{figure*}[t]
  \centering 
  \subfigure[Classification Macro Average F1]{ 
    \includegraphics[width=0.48\linewidth]{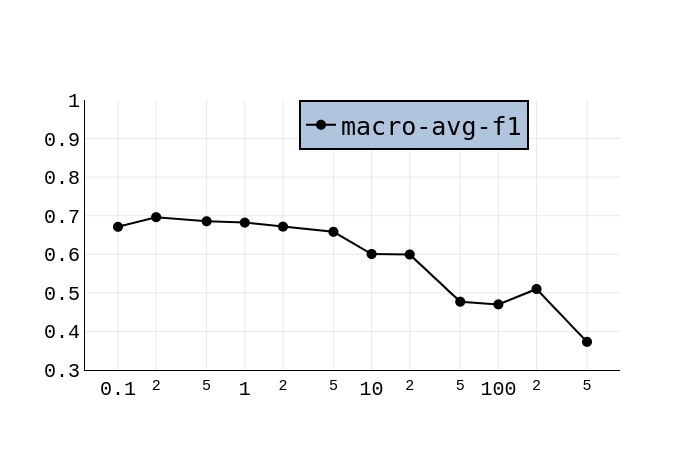}}
   \subfigure[comprehensiveness and sufficiency]{ 
     \includegraphics[width=0.48\linewidth]{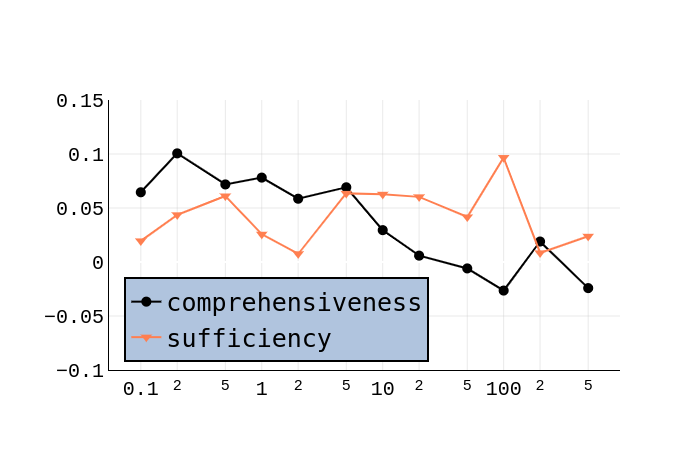}}
   \subfigure[AUPRC]{ 
     \includegraphics[width=0.48\linewidth]{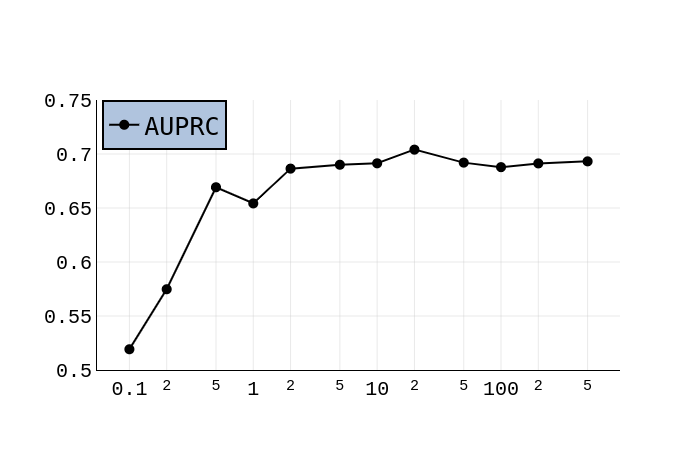}}
  \subfigure[Macro F1]{ 
    \includegraphics[width=0.48\linewidth]{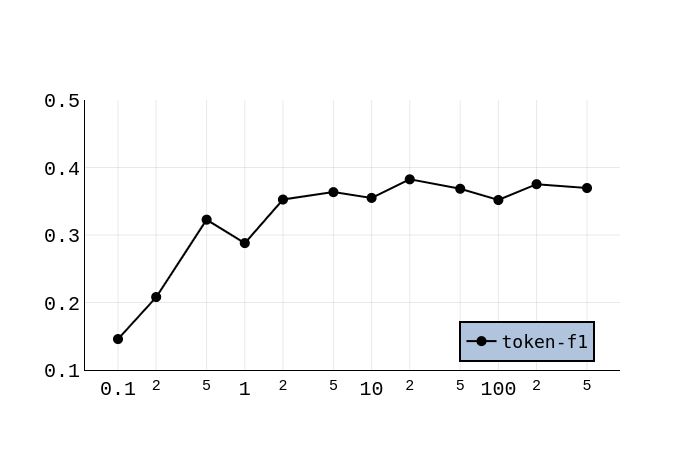}}
  \subfigure[$\lambda$-selection criteria for \mtlhard ]{ 
    \includegraphics[width=0.48\textwidth]{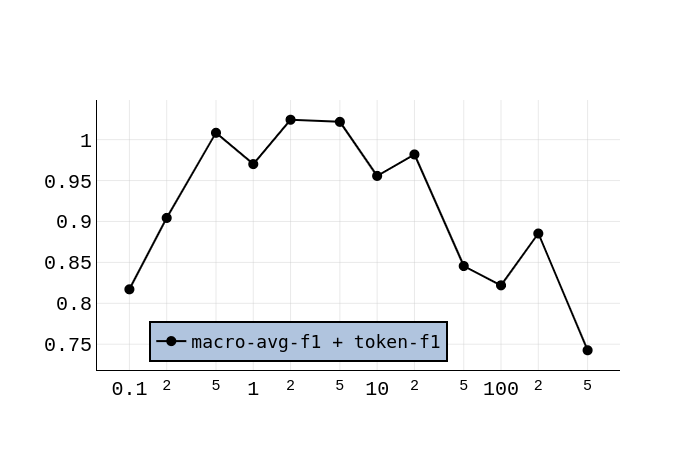}}
  \subfigure[$\lambda$-selection criteria for \mtlsoft]{ 
    \includegraphics[width=0.48\textwidth]{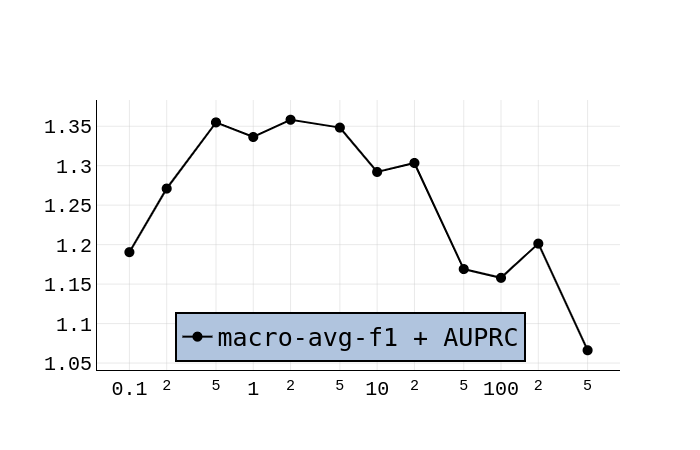}}    
    \caption{Performance of task (a), explanation (b, c, d) and our $\lambda$ selection criteria for \mtlhard~and \mtlsoft~(e, f) with $\lambda$ (log-scale)  on the validation set of \multirc. Models for parameter-sweeping is trained on 25\% of the training set.}
  \label{fig:multirc_lambda_sweep}
\end{figure*}

\section{Training time of our \approach}
The training time of our approach depends highly on the size of the dataset, batch size used in training and computational load of our machine. 
Therefore the data presented in table~\ref{tab:training_time} is a very rough estimation. Other configurations regarding training setup are presented in \ref{sec:parameter_setup}.
The important thing to note that all our approaches where trained for the same number of 10 epochs, with patience=3 epochs for a fair comparison.
Our competitors~\cite{lei2016rationalizing,deyoung2019eraser} was trained for 20 epochs with early stopping with patience of 5 epochs;~\cite{lehman2019inferring} was trained for 50 epochs 10 patience; and Bert-to-Bert was trained for  10 epochs (as reported in~\cite{deyoung2019eraser}).

\begin{table*}[]
    \centering
    \resizebox{\linewidth}{!}{
    \begin{tabular}{c|cccc}
    \toprule
            & \expstg & \mtltask & \mtst & \cls \\
            \hline
    \movie  & 9m   & 31m      & 7m   &5m    \\
    \fever  & 5h55m&13h22m    & 4h32m&3h32m \\
    \multirc& 1h18m& 2h49m    & 55m  &1h39m \\
    \bottomrule
    \end{tabular}}
    \caption{Roughly estimated training time}
    \label{tab:training_time}
\end{table*}
