# Supplementary material for: Explain and Predict, and then Predict Again
Source: arXiv:2101.04109 source file (2021-02-04)
Supplement: Supplementary file 2 [file a.appendix.backup.tex]

\clearpage
\appendix
\section{Statistics of the explanations}
Three statistics of machine-generated and human-annotated by human explanations are presented in the table \ref{tab:avg_rats_len}. By macro average length (Macro Avg Length), it means at first averaging the length of explanation/annotation intervals within each instance and then averaging them across all instances. The $P_{EXP}$ represents precision and the $R_{EXP}$ stands for recall of the machine-generated explanation given human annotation.
\begin{table}[]
    \centering
    \resizebox{0.98\linewidth}{!}{
    \begin{tabular}{lccc}
        \toprule
            & Macro Avg Length & $P_{EXP}$ & $R_{EXP}$ \\
        \hline
        \textbf{\movie}\\
        \exptask & 4.795 & 0.699 & 0.129 \\
        \mtlhard(\mtltask) & 4.091 & 0.666 & 0.096 \\
        \human & 24.225 & 1.000 & 1.000 \\
        \hline
        \textbf{\fever}\\
        \exptask & 28.739 & 0.815 & 0.747 \\
        \mtlhard(\mtltask) & 27.142 & 0.814 & 0.741 \\
        \human & 29.044 & 1.000 & 1.000\\
        \hline
        \textbf{\multirc}\\
        \exptask & 31.228 & 0.629 & 0.627 \\
        \mtlhard(\mtltask) & 25.457 & 0.648 & 0.577 \\
        \human & 21.603 & 1.000 & 1.000 \\
        \bottomrule
    \end{tabular}
    }
    \caption{Statistics of the machine-generated and human-annotated explanations}
    \label{tab:avg_rats_len}
\end{table}

The table \ref{tab:jaccards_me_he} describes the concordance between machine-generated explanation and human annotation. From the table, we can see the overlap between the human and machine rationale is relatively limited. We can also observe such phenomena with help of anecdotal examples of all three different rationales. Some of such examples are presented in the table~\ref{tab:anecdotal}. Notifiable that for some instances, the instance from \fever presented in table~\ref{tab:anecdotal} for example, the machine-generated explanation (that Emma Watson was born in 1990) could be a piece of alternative evidence refuting the statement (that Emma Watson was killed in 1990).

\begin{table}[]
    \centering
    \resizebox{0.98\linewidth}{!}{
    \begin{tabular}{cccc}
    \toprule
               & Jaccard similarity & One-way Jaccard \\
        \hline
        \textbf{\movie}\\ 
            \exptask & 0.120 & 0.699\\
            \mtlhard & 0.090 & 0.666\\
        \hline
        \textbf{\fever}\\
            \exptask & 0.705 & 0.815\\
            \mtlhard & 0.700 & 0.813\\
        \hline
        \textbf{\multirc}\\
            \exptask & 0.495 & 0.629\\
            \mtlhard & 0.468 & 0.648\\
    \bottomrule
    \end{tabular}}
    \caption{Jaccard similarity and One-way Jaccard (precision of machine rationale) between machine selected rationale and human annotation}
    \label{tab:jaccards_me_he}
\end{table}

\begin{table*}[]
    \centering
    \begin{tabular}{p{0.08\linewidth}|p{0.27\linewidth}|p{0.27\linewidth}|p{0.27\linewidth}}
    \toprule
         &  \human & \exptask & \mtlhard \\
         \hline
    \movie
        & ... "She's All That" has \textbf{the dubious distinction of being the worst movie I've seen so far this year}. And quite frankly, \textbf{I doubt I'll see anything equally bad. (at least, I *hope* I don't see anything equally bad)}. "She's All That" tells ... popular. \textbf{That, right there , is problem \#1. How many times have we seen this storyline}?... 
        & ... "She's All That" has \textbf{the dubious} distinction \textbf{of being the worst movie I've seen so far this year}. And quite frankly, I doubt I'll see anything equally bad. (at least, I *hope* I don't see anything equally bad). "She's All That" tells ... popular. That, right there , is problem \#1. How many times have we seen this storyline?... 
        & ... "She's All That" has the dubious distinction \textbf{of being the worst movie I}'\textbf{ve seen so far} this \textbf{year}. And quite frankly, I doubt I'll see anything equally \textbf{bad}. (at least, I *hope* I don't see anything equally bad). "She's All That" tells ... popular. That, right there , is problem \#1. How many times have we seen this storyline?...\\
    \hline
    \fever{}
        & Q: Emma Watson was killed in 1990.\newline
          Doc: Emma Charlotte Duerre Watson (born 15 april 1990) is a French-British actress, model, and activist. Born in Paris ... previously. \textbf{Watson appeared in all eight Harry Potter films from 2001 to 2011, earning worldwide fame, critical accolades, and around \$60 million}...
        & Q: Emma Watson was killed in 1990.\newline
          Doc: \textbf{Emma Charlotte Duerre Watson (born 15 april 1990) is a French-British actress, model, and activist.} Born in Paris ... previously. Watson appeared in all eight Harry Potter films from 2001 to 2011, earning worldwide fame, critical accolades, and around \$60 million...
        & Q: Emma Watson was killed in 1990.\newline
          Doc: \textbf{Emma Charlotte Duerre Watson (born 15 april 1990) is a French-British actress, model, and activist.} Born in Paris ... previously. \textbf{Watson appeared in} all eight Harry Potter films \textbf{from 2001 to 2011, earning worldwide fame, critical accolades, and around \$60 million.}...\\
    \hline
    \multirc{}
        & Q: What did the judge tell Mr. Thorndike about the law ?\newline
        A: It was unjust\newline
        Doc: ...The judge leaned over his desk and shook Mr. Thorndike by the hand. Then he made a speech. ... He purposely spoke in a loud voice, and every one stopped to listen. \textbf{"The law, Mr. Thorndike, is not vindictive," he said. "It wishes only to be just. nor can it be swayed by wealth or political or social influences.}...
        & Q: What did the judge tell Mr. Thorndike about the law ?\newline
        A: It was not vindictive.\newline
        Doc: ...\textbf{The judge leaned over his desk and shook Mr. Thorndike by the hand.} Then he made a speech. ... He purposely spoke in a loud voice, and every one stopped to listen. \textbf{"The law, Mr. Thorndike, is not vindictive," he said.} "It wishes only to be just. nor can it be swayed by wealth or political or social influences...
        & Q: What did the judge tell Mr. Thorndike about the law ?\newline
        A: It was not vindictive.\newline
        Doc: ...\textbf{The judge leaned over his desk and shook Mr. Thorndike by the hand.} Then he made a speech. ... He purposely spoke in a loud voice, and every one stopped to listen. \textbf{"The law, Mr. Thorndike, is not vindictive," he said. "It wishes only to be just. nor can it be swayed by wealth or political or social influences.}...\\
    \bottomrule
    \end{tabular}
    \caption{Examples of rationale annotations. All instances are predicted correctly in the auxiliary output of the MTL model}
    \label{tab:anecdotal}
\end{table*}


\section{Details on the effect of $\lambda$}
\label{sec:detailed-lambda-sweep}
% In Section~\ref{sec:eval}, we report the performance of both auxiliary predictor and the explainer of our proposed approaches \mtlhard for the best performing values of $\lambda$. The concept 'best performing' refers to the highest score by the summation of auxiliary and explainer performance (for \mtlhard they are Macro average F1 of the auxiliary predictor and the token F1 of the explainer, while for the soft-selection variation discussed in \ref{sec:analysis})/ Table~\ref{tab:hard_task_performance} and~\ref{table:task_explanation_result_soft} compare the performance of the proposed approaches with the hard and soft-selection based baselines respectively. However, we observe that the performance of the task and explanation vary a lot with the parameter $\lambda$. Figures~\ref{fig:fever_lambda_sweep}---\ref{fig:multirc_lambda_sweep} show the performance variation of \mtlhard for each of the three datasets(\fever, \movie~and \multirc).

% We now analyze the impact of $\lambda$ on the task and explanation performance in Figure~\ref{fig:fever_lambda_sweep} on the \fever{} dataset, given that similar trend is observed for other datasets.  
% As expected, we observe an inverse relationship between the performance of task and explanation i.e., the performance of the task decreases, and explanation increases with the increased value of $\lambda$ shown clearly in the figure.
% Interestingly, there is a stable plateau in the range $\lambda \in [1,50]$ that exhibits low variability performance task and explanation performance.
% However, the task performance deteriorates rapidly after $\lambda\geq50$ (or low weightage to task-specific loss) indicating that optimizing purely for explanation generation deteriorates task performance. 

% \begin{figure*}[tb] 
%   \centering 
%   \subfigure[\textbf{Classification Macro Average F1}]{ 
%     \label{fig:subfig:acc}
%     \includegraphics[width=0.48\linewidth]{figs/task_f1.pdf}}
%   \subfigure[\textbf{Explanation Macro F1}]{ 
%     \label{fig:subfig:macro_f1}
%     \includegraphics[width=0.48\linewidth]{figs/hard_exp_metric.pdf}}
%     \caption{Performance variation of task (a) and explanation (macro token/IOU-F1) (b) of \methodindv{} with $\lambda$ (log-scale) on the first 10\% \fever{} dataset. Here we can see the obvious contradiction between classification and explanation along the $\lambda$ increases...\todo{consider merging plots.}}
%   \label{fig:lambda-sweep_1} 
% \end{figure*}

\begin{figure*}[tb]
  \centering 
  \subfigure[Classification Macro Average F1]{ 
    \includegraphics[width=0.48\textwidth]{figs/lambda_sweep/fever_gru_val_train_on_portion_0_1_macro_avg_f1.png}}
  \subfigure[comprehensiveness and sufficiency]{ 
    \includegraphics[width=0.48\textwidth]{figs/lambda_sweep/fever_gru_val_train_on_portion_0_1_cs.png}}
  \subfigure[AUPRC]{ 
    \includegraphics[width=0.48\textwidth]{figs/lambda_sweep/fever_gru_val_train_on_portion_0_1_auprc.png}}
  \subfigure[Macro F1]{ 
    \includegraphics[width=0.48\textwidth]{figs/lambda_sweep/fever_gru_val_train_on_portion_0_1_iou_token_f1.png}}
  \caption{Performance variation of task (a) and explanation (b, c, d) $\lambda$ (log-scale) on the validation set of \fever. Models for sweeping is trained over 10\% of the training set.}
  \label{fig:fever_lambda_sweep}
\end{figure*}

\begin{figure*}[t]
  \centering 
  \subfigure[Classification Macro Average F1]{ 
    \includegraphics[width=0.48\linewidth]{figs/lambda_sweep/movies_gru_val_train_on_portion_0_macro_avg_f1.png}}
   \subfigure[comprehensiveness and sufficiency]{ 
     \includegraphics[width=0.48\linewidth]{figs/lambda_sweep/movies_gru_val_train_on_portion_0_cs.png}}
   \subfigure[AUPRC]{ 
     \includegraphics[width=0.48\linewidth]{figs/lambda_sweep/movies_gru_val_train_on_portion_0_auprc.png}}
  \subfigure[Macro F1]{ 
    \includegraphics[width=0.48\linewidth]{figs/lambda_sweep/movies_gru_val_train_on_portion_0_iou_token_f1.png}}
    \caption{Performance of task (a) and explanation (b) $\lambda$ (log-scale) on the validation set of \movie.}
  \label{fig:movie_lambda_sweep}
\end{figure*}

\begin{figure*}[t]
  \centering 
  \subfigure[Classification Macro Average F1]{ 
    \includegraphics[width=0.48\linewidth]{figs/lambda_sweep/multirc_gru_val_train_on_portion_0_4_macro_avg_f1.png}}
   \subfigure[comprehensiveness and sufficiency]{ 
     \includegraphics[width=0.48\linewidth]{figs/lambda_sweep/multirc_gru_val_train_on_portion_0_4_cs.png}}
   \subfigure[AUPRC]{ 
     \includegraphics[width=0.48\linewidth]{figs/lambda_sweep/multirc_gru_val_train_on_portion_0_4_auprc.png}}
  \subfigure[Macro F1]{ 
    \includegraphics[width=0.48\linewidth]{figs/lambda_sweep/multirc_gru_val_train_on_portion_0_4_iou_token_f1.png}}
    \caption{Performance variation of task (a) and explanation (b) $\lambda$ (log-scale) on the validation set of \multirc. Models for sweeping is trained over 25\% of the training set.}
  \label{fig:multirc_lambda_sweep}
\end{figure*}

\section{Training time of our \approach}
The training time of our approach depends highly on the size of the dataset, batch size used in training and computational load of our machine. Therefore the data presented in table~\ref{tab:training_time} is a very rough estimation. Other configurations regarding training setup are presented in \ref{sec:parameter_setup}.

\begin{table*}[]
    \centering
    \resizebox{\linewidth}{!}{
    \begin{tabular}{c|cccc}
    \toprule
            & \expstg & \mtltask & \mtst & \cls \\
            \hline
    \movie  & 9m   & 31m      & 7m   &5m    \\
    \fever  & 5h55m&13h22m    & 4h32m&3h32m \\
    \multirc& 1h18m& 2h49m    & 55m  &1h39m \\
    \bottomrule
    \end{tabular}}
    \caption{Roughly estimated training time}
    \label{tab:training_time}
\end{table*}
% \begin{figure*}
% \parbox{\textwidth}{
% \center
% \subfloat[{\bf Classification Macro Average F1}]{\includegraphics[width=0.48\textwidth]{figs/lambda_sweep/fever_gru_val_train_on_portion_0_1_macro_avg_f1.png}}
% \hfil
% \subfloat[{\bf comprehensiveness and sufficiency}]{\includegraphics[width=0.48\textwidth]{figs/lambda_sweep/fever_gru_val_train_on_portion_0_1_cs.png}}}

% \parbox{\textwidth}{
% \center
% \subfloat[{\bf AUPRC}]{\includegraphics[width=0.48\textwidth]{figs/lambda_sweep/fever_gru_val_train_on_portion_0_1_auprc.png}}
% \hfil
% \subfloat[{\bf Macro F1}]{\includegraphics[width=0.48\textwidth]{figs/lambda_sweep/fever_gru_val_train_on_portion_0_1_iou_token_f1.png}}
% \caption{{\bf Performance of \textit{cls} and \textit{exp} task in \methodindv w.r.t. 6 metrics on log-scale variation of $\lambda$ on the top 10\% of~\fever. Horizontal lines and curves sharing same line type in each sub-figure correspond to the same metric, where the horizontal lines are the highest (for sufficiency the lowest) scores of each metrics out of all baseline models.}}
% \label{fig:indv1}}
% %\vspace*{-6mm}
% \end{figure*}
% %\FloatBarrier

% \begin{figure*}[tb]
% %\parbox{\textwidth}{
% \center
% \subfloat[{\bf Classification Macro Average F1}]{\includegraphics[width=0.48\textwidth]{figs/lambda_sweep/fever_gru_val_train_on_portion_0_1_macro_avg_f1.png}}
% \hfil
% \subfloat[{\bf comprehensiveness and sufficiency}]{\includegraphics[width=0.48\textwidth]{figs/lambda_sweep/fever_gru_val_train_on_portion_0_1_cs.png}}%}
% \caption{{\bf Performance of \textit{cls} and \textit{exp} task in \methodindv w.r.t. 6 metrics on log-scale variation of $\lambda$ on the top 10\% of~\fever. Horizontal lines and curves sharing same line type in each sub-figure correspond to the same metric, where the horizontal lines are the highest (for sufficiency the lowest) scores of each metrics out of all baseline models.}}
% \label{fig:indv1}
% \end{figure*}

% \begin{figure*}[tb]
% \center
% \subfloat[{\bf AUPRC}]{\includegraphics[width=0.48\textwidth]{figs/lambda_sweep/fever_gru_val_train_on_portion_0_1_auprc.png}}
% \hfil
% \subfloat[{\bf Macro F1}]{\includegraphics[width=0.48\textwidth]{figs/lambda_sweep/fever_gru_val_train_on_portion_0_1_iou_token_f1.png}}
% \caption{{\bf Performance of \textit{cls} and \textit{exp} task in \methodindv w.r.t. 6 metrics on log-scale variation of $\lambda$ on the top 10\% of~\fever. Horizontal lines and curves sharing same line type in each sub-figure correspond to the same metric, where the horizontal lines are the highest (for sufficiency the lowest) scores of each metrics out of all baseline models.}}
% \label{fig:indv1}%}
% %\vspace*{-6mm}
% \end{figure*}






% \if 0
% Figures in this section of the appendix are supplementary to the section \ref{sec:results}. This section contains 6 figures, 3 or 4 sub-figures each, depicting the variation w.r.t. 5 or 6 metrics (\textbf{Macro F1}, \textbf{AUPRC}\footnote{We don't have \textbf{AUPRC} for \methodspan}, \textbf{Comprehensiveness}, \textbf{Sufficiency}, \textbf{IOU F1}, \textbf{Token F1}) on 3 datasets (\fever, \movie~and \multirc) for 2 different methods (\methodindv~and \methodspan).
% \fi

% \begin{figure*}[tb]
% \parbox{\textwidth}{
% \center
% \subfloat[{\bf Classification Macro Average F1}]{\includegraphics[width=0.48\textwidth]{figs/lambda_sweep/fever_gru_val_train_on_portion_0_1_macro_avg_f1.png}}
% \hfil
% \subfloat[{\bf comprehensiveness and sufficiency}]{\includegraphics[width=0.48\textwidth]{figs/lambda_sweep/fever_gru_val_train_on_portion_0_1_cs.png}}}

% \parbox{\textwidth}{
% \center
% \subfloat[{\bf AUPRC}]{\includegraphics[width=0.48\textwidth]{figs/lambda_sweep/fever_gru_val_train_on_portion_0_1_auprc.png}}
% \hfil
% \subfloat[{\bf Macro F1}]{\includegraphics[width=0.48\textwidth]{figs/lambda_sweep/fever_gru_val_train_on_portion_0_1_iou_token_f1.png}}
% \caption{{\bf Performance of \textit{cls} and \textit{exp} task in \methodindv w.r.t. 6 metrics on log-scale variation of $\lambda$ on the top 10\% of~\fever. Horizontal lines and curves sharing same line type in each sub-figure correspond to the same metric, where the horizontal lines are the highest (for sufficiency the lowest) scores of each metrics out of all baseline models.}}
% \label{fig:indv1}}
% %\vspace*{-6mm}
% \end{figure*}

% \todo{I guess you can use parbox}


% \begin{figure*}[t]
%   \centering 
%   \subfigure[Classification Macro Average F1]{ 
%     \includegraphics[width=0.48\linewidth]{figs/lambda_sweep/fever_rnr_val_train_on_portion_0_1_macro_avg_f1.png}}
%   \subfigure[comprehensiveness and sufficiency]{ 
%     \includegraphics[width=0.48\linewidth]{figs/lambda_sweep/fever_rnr_val_train_on_portion_0_1_cs.png}}
%   \subfigure[Macro F1]{ 
%     \includegraphics[width=0.48\linewidth]{figs/lambda_sweep/fever_rnr_val_train_on_portion_0_1_iou_token_f1.png}}
    
%  \caption{{\bf Performance variation of task (a) and explanation (b,c) of \methodspan{} with $\lambda$ (log-scale) on the first 10\% \fever{} dataset.}}
%   %\caption{{\bf Performance of \textit{cls} and \textit{exp} task in \methodspan w.r.t. 5 metrics on log-scale variation of $\lambda$ on the top 10\% data of~\fever. Horizontal lines and curves sharing same line type in each sub-figure correspond to the same metric, where the horizontal lines are the highest (for sufficiency the lowest) scores of each metrics out of all baseline models.}}
%   \label{fig:span1}
% \end{figure*}



% \begin{figure*}[t]
%   \centering 
%   \subfigure[Classification Macro Average F1]{ 
%     \includegraphics[width=0.48\linewidth]{figs/lambda_sweep/movies_rnr_val_train_on_portion_0_macro_avg_f1.png}}
%   \subfigure[comprehensiveness and sufficiency]{ 
%     \includegraphics[width=0.48\linewidth]{figs/lambda_sweep/movies_rnr_val_train_on_portion_0_cs.png}}
%   \subfigure[Macro F1]{ 
%     \includegraphics[width=0.48\linewidth]{figs/lambda_sweep/movies_rnr_val_train_on_portion_0_iou_token_f1.png}}
%   \caption{{\bf Performance variation of task (a) and explanation (b,c) of \methodspan{} with $\lambda$ (log-scale) on the \movie.}}
%   %\caption{{\bf Performance of \textit{cls} and \textit{exp} task in \methodspan w.r.t. 5 metrics on log-scale variation of $\lambda$ on~\movie. Horizontal lines and curves sharing same line type in each sub-figure correspond to the same metric, where the horizontal lines are the highest (for sufficiency the lowest) scores of each metrics out of all baseline models.}}
%   \label{fig:span2}
% \end{figure*}



% \begin{figure*}[t]
%   \centering 
%   \subfigure[Classification Macro Average F1]{ 
%     \includegraphics[width=0.48\linewidth]{figs/lambda_sweep/multirc_rnr_val_train_on_portion_0_4_macro_avg_f1.png}}
%   \subfigure[comprehensiveness and sufficiency]{ 
%     \includegraphics[width=0.48\linewidth]{figs/lambda_sweep/multirc_rnr_val_train_on_portion_0_4_cs.png}}
%   \subfigure[Macro F1]{ 
%     \includegraphics[width=0.48\linewidth]{figs/lambda_sweep/multirc_rnr_val_train_on_portion_0_4_iou_token_f1.png}}
%   \caption{{\bf Performance variation of task (a) and explanation (b,c) of \methodspan{} with $\lambda$ (log-scale) on the first 25\% \multirc{} dataset.}}
%   %\caption{{\bf Performance of \textit{cls} and \textit{exp} task in \methodspan w.r.t. 5 metrics on log-scale variation of $\lambda$ on top 25\% of~\movie. Horizontal lines and curves sharing same line type in each sub-figure correspond to the same metric, where the horizontal lines are the highest (for sufficiency the lowest) scores of each metrics out of all baseline models.}}
%   \label{fig:span3}
% \end{figure*}


% \section{Example Tabble for Zijian}


% \newcommand{\senlabel}{\textsc{BERT-3S}}
% \newcommand{\qa}{\textsc{QA-Ranker}}
% \newcommand{\qalabel}{\textsc{Qa-DocRank}}
% \newcommand{\qaweaklabel}{\textsc{QA-Full-DOCRANK}}
% \newcommand{\qaweaksupervised}{\textsc{QA-Weak-Supervised}}
% \newcommand{\qamodel}{\textsc{QA-Model}}
% \newcommand{\passagererank}{\textsc{Passage-Rerank}}
% %\newcommand{\clam}{\textsc{Classification And Aggregation based Neural Ranking Models}}
% \newcommand{\clam}{\textsc{BERT based Rankers}}
% \newcommand{\doclabel}{\textsc{Doc-Labelled}}
% \newcommand{\msm}{\textsc{MS Marco}}
% \newcommand{\trecdl}{\textsc{TREC-DL}}
% \newcommand{\robust}{\textsc{Robust04}}
% \newcommand{\core}{\textsc{Core17}}
% \newcommand{\clueweb}{\textsc{ClueWeb09}}

% \newcommand{\bm}{\textsc{BM25}}
% \newcommand{\drmm}{\textsc{Drmm}}
% \newcommand{\pacr}{\textsc{Pacrr}}
% \newcommand{\mpcos}{\textsc{MatchPyramid}}
% \newcommand{\pdrmm}{\textsc{PacrrDrmm}}
% \newcommand{\nrpf}{\textsc{Nprf-Drmm}}
% \newcommand{\indri}{\textsc{Indri-QL}}
% \newcommand{\bs}{\textsc{Base-Scorer}}



% \begin{table*}[tb]
% \centering
% \resizebox{\textwidth}{!}{
% \begin{tabular}{lcccccccccccc} 
% %\hline
% \toprule
% \multirow{2}{*}{\textbf{Method}} & \multicolumn{3}{c}{\textbf{\robust}}  & \multicolumn{3}{c}{\textbf{\trecdl}} & \multicolumn{3}{c}{\textbf{\core}} & \multicolumn{3}{c}{\textbf{\clueweb}}                      \\
% \cmidrule(lr){2-4}
% \cmidrule(lr){5-7}
% \cmidrule(lr){8-10}
% \cmidrule(lr){11-13}
%                           &  \textbf{MAP} & \textbf{nDCG20} & \textbf{P@20} & \textbf{MAP} & \textbf{nDCG20} &  \textbf{P@20} & \textbf{MAP} & \textbf{nDCG20} &  \textbf{P@20} & \textbf{MAP} & \textbf{nDCG20} &  \textbf{P@20} \\ %\hline
%                      \midrule
                     
% \textbf{QL Model} & 0.240 & $0.403^*$ & 0.347 & 0.227 & $0.298^*$ & 0.028 & 0.203 & $0.395^*$ & 0.474 & 0.165 & $0.277^*$ & 0.331 \\
% % \cmidrule(lr){1-13}
% \bf \pdrmm & 0.263 & 0.445 & 0.374 & 0.277 & $0.347^*$ & 0.033 & 0.215 & $0.418^*$ & 0.497 & 0.169 & $0.285^*$ & 0.336 \\
% % \cmidrule(lr){1-13}
% % \bf \mpcos & 0.189 & 0.332 & 0.276 & 0.183 & 0.251 & 0.025 \\
% %  \bf \drmm & 0.257 & 0.410 & 0.352 & 0.216 & 0.287 & 0.028 \\
% %   \bf \pacr & 0.260 & 0.442 & 0.372 & 0.265 & 0.340 & 0.030 \\
% %   \bf \pdrmm & 0.263 & 0.445 & 0.374 & 0.277 & 0.347 & 0.033 \\
% % \cmidrule(lr){1-7}

% %   \bf \doclabel{}-Limited & 0.233 & $0.377^*$ & 0.333 & 0.281 & $0.363^*$ & 0.033 & 0.208 & $0.347^*$ & 0.425 & 0.173 & $0.29^*$ & 0.333 \\ 

%   \bf \doclabel{}     & 0.256 & $0.432^*$ & 0.372 & 0.297 & $0.378^*$ & 0.033 & 0.229 & 0.438 & 0.525 & 0.173 & $0.293^*$ & 0.347 \\
% % \cmidrule(lr){1-13}
%   \bf \senlabel{} & {\bf 0.290} & {\bf 0.477} & {\bf 0.409} & {\bf 0.314} & {\bf 0.393} & {\bf 0.033} & {\bf 0.258} & {\bf 0.475} & {\bf 0.570} & {\bf 0.185} & {0.315} & {0.366} \\
% % \cmidrule(lr){1-13}
%   \bf \qalabel{} &  0.288 & 0.459 & 0.404 & {\bf 0.315} & {\bf 0.394} & {\bf 0.033} & {0.233} & {0.467} & { 0.545} & {0.175} & {$0.312^*$} & {0.354} \\
% % \cmidrule(lr){1-13}
%   \bf QL+\qalabel{} &  0.288 & 0.459 & 0.404 & {\bf 0.315} & {\bf 0.394} & {\bf 0.033} & {0.243} & {0.473} & { 0.552} & {\bf 0.189} & {\bf 0.331} & {\bf 0.372} \\
% %\\
% \bottomrule
% \end{tabular}}
% \caption{{\bf title here}}

% \label{tab:model_eval}
% % \vspace{-5mm}
% \end{table*}






% \begin{table*}[]
%     \centering
%     \begin{tabular}{p{0.08\linewidth}|p{0.27\linewidth}|p{0.27\linewidth}|p{0.27\linewidth}}
%     \toprule
%          &  \human & \exptask & \mtlhard \\
%          \hline
%     \movie
%         & Ah, and 1999 was going along so well, too. "She's All That" has \textbf{the dubious distinction of being the worst movie I've seen so far this year}. And quite frankly, \textbf{I doubt I'll see anything equally bad. (at least, I *hope* I don't see anything equally bad)}. "She's All That" tells the story of the most popular guy in school (played by freddie prinze Jr.) who accepts a bet to transform the geekiest girl in school (Rachel Leigh Cook) into the most popular. \textbf{That, right there , is problem \#1. How many times have we seen this storyline}?... 
%          & Ah, and 1999 was going along so well, too. "She's All That" has \textbf{the dubious} distinction \textbf{of being the worst movie I've seen so far this year}. And quite frankly, I doubt I'll see anything equally bad. (at least, I *hope* I don't see anything equally bad). "She's All That" tells the story of the most popular guy in school (played by Freddie Prinze Jr.) who accepts a bet to transform the geekiest girl in school (Rachel Leigh Cook) into the most popular. That, right there , is problem \#1. How many times have we seen this storyline?... 
%          & Ah, and 1999 was going along so well, too. "She's All That" has the dubious distinction \textbf{of being the worst movie I}'\textbf{ve seen so far} this \textbf{year}. And quite frankly, I doubt I'll see anything equally \textbf{bad}. (at least, I *hope* I don't see anything equally bad). "She's All That" tells the story of the most popular guy in school (played by Freddie Prinze Jr.) who accepts a bet to transform the geekiest girl in school (Rachel Leigh Cook) into the most popular. That, right there , is problem \#1. How many times have we seen this storyline?...\\
%     \fever{}
%         & Q: Emma Watson was killed in 1990.\newline
%           Doc: Emma Charlotte Duerre Watson (born 15 april 1990) is a French-British actress, model, and activist. Born in Paris and brought up in Oxfordshire, Watson attended the Dragon School and trained as an actress at the Oxford Branch of Stagecoach Theatre Arts. She rose to prominence after landing her first professional acting role as Hermione Granger in the Harry Potter film series, having acted only in school plays previously. \textbf{Watson appeared in all eight Harry Potter films from 2001 to 2011, earning worldwide fame, critical accolades, and around \$60 million. Watson continued to work outside of the Harry Potter films, lending her voice to the tale of Despereaux (2008) and appearing in the 2007 television adaptation of the novel Ballet Shoes}...
%         & Q: Emma Watson was killed in 1990.\newline
%           Doc: \textbf{Emma Charlotte Duerre Watson (born 15 april 1990) is a French-British actress, model, and activist.} Born in Paris and brought up in Oxfordshire, Watson attended the Dragon School and trained as an actress at the Oxford Branch of Stagecoach Theatre Arts. She rose to prominence after landing her first professional acting role as Hermione Granger in the Harry Potter film series, having acted only in school plays previously. Watson appeared in all eight Harry Potter films from 2001 to 2011, earning worldwide fame, critical accolades, and around \$60 million. Watson continued to work outside of the Harry Potter films, lending her voice to the tale of Despereaux (2008) and appearing in the 2007 television adaptation of the novel Ballet Shoes...
%         & Q: Emma Watson was killed in 1990.\newline
%           Doc: \textbf{Emma Charlotte Duerre Watson (born 15 april 1990) is a French-British actress, model, and activist.} Born in Paris and brought up in Oxfordshire, Watson attended the Dragon School and trained as an actress at the Oxford Branch of Stagecoach Theatre Arts. She rose to prominence after landing her first professional acting role as Hermione Granger in the Harry Potter film series, having acted only in school plays previously. \textbf{Watson appeared in} all eight Harry Potter films \textbf{from 2001 to 2011, earning worldwide fame, critical accolades, and around \$60 million.} Watson continued to work outside of the Harry Potter films, lending her voice to the tale of Despereaux (2008) and appearing in the 2007 television adaptation of the novel Ballet Shoes...
%     \bottomrule
%     \end{tabular}
%     \caption{Examples on rationales}
%     \label{tab:anecdotal}
% \end{table*}
